# Supplementary material for: SemEval-2023 Task 2: Fine-grained Multilingual Named Entity Recognition (MultiCoNER 2)
Source: arXiv:2305.06586 source file (2023-05-25)
Supplement: Supplementary file 2 [file f_r_en.tex]

\begin{table*}[!hbtp]
\resizebox{\textwidth}{!}{%
\begin{tabular}{c lllllll}

\toprule

\textbf{Rank} & 
\textbf{Team} & 
\textbf{Clean Subset F1} & 
\textbf{Noisy Subset F1} & 
\textbf{Entity Noise F1} &
\textbf{Context Noise F1} &  
\textbf{Macro F1}\\ 
\addlinespace[0.2cm]
\midrule

1 & DAMO-NLP & 88.13 & 79.76 & 79.07 & 86.30 & 85.53 \\
2 & {\small Samsung Research China - Beijing} & 85.36 & 77.94 & 77.33 & 83.74 & 83.09 \\
3 & PAI & 86.16 & 65.41 & 63.23 & 84.74 & 80.00 \\
4 & CAIR-NLP & 81.29 & 74.89 & 74.58 & 77.83 & 79.33 \\
5 & KDDIE & 80.08 & 73.50 & 73.03 & 78.05 & 78.06 \\
6 & SRCB & 79.74 & 66.21 & 65.06 & 76.56 & 75.62 \\
7 & IXA/Cogcomp & 76.64 & 64.36 & 63.81 & 69.59 & 72.82 \\
8 & USTC-NELSLIP & 74.87 & 65.76 & 65.35 & 69.18 & 72.15 \\
9 & NLPeople & 76.00 & 62.23 & 60.93 & 74.52 & 71.81 \\
10 & BizNER & 72.12 & 66.64 & 66.32 & 69.65 & 70.44 \\
11 & Sakura & 72.86 & 64.06 & 63.79 & 66.39 & 70.16 \\
12 & RIGA & 70.74 & 66.07 & 65.84 & 68.23 & 69.30 \\
13 & CodeNLP & 66.04 & 57.84 & 57.58 & 60.17 & 63.51 \\
14 & Sartipi-Sedighin & 67.10 & 54.56 & 53.68 & 62.86 & 63.25 \\
15 & IITD & 67.52 & 53.59 & 52.82 & 60.47 & 63.21 \\
16 & garNER & 65.25 & 56.96 & 56.73 & 58.90 & 62.73 \\
17 & FII\_Better & 65.67 & 52.74 & 51.87 & 60.60 & 61.75 \\
18 & D2KLab & 64.72 & 53.54 & 53.12 & 57.24 & 61.29 \\
19 & silp\_nlp & 62.59 & 56.96 & 56.91 & 57.22 & 60.85 \\
20 & Ertim & 61.85 & 52.78 & 52.76 & 52.75 & 59.03 \\
21 & MEERQAT-IRIT & 60.46 & 54.72 & 54.68 & 55.03 & 58.70 \\
22 & LSJSP & 60.67 & 50.48 & 50.44 & 50.59 & 57.51 \\
23 & RGAT & 61.29 & 47.15 & 46.56 & 52.04 & 56.91 \\
24 & CLaC & 57.68 & 49.06 & 48.91 & 50.26 & 55.05 \\
25 & L3i++ & 55.87 & 46.70 & 46.47 & 48.68 & 53.00 \\
26 & VBD\_NLP & 57.00 & 42.44 & 41.45 & 51.06 & 52.65 \\
27 & LLM-RM & 54.73 & 46.30 & 46.17 & 47.45 & 52.08 \\
28 & Minanto & 53.43 & 47.00 & 47.03 & 46.48 & 51.47 \\
29 & SAB & 54.28 & 44.96 & 44.82 & 46.16 & 51.41 \\
30 & ShathaTaymaaTeam & 52.34 & 44.78 & 45.09 & 41.67 & 50.02 \\
31 & azaad@BND & 50.09 & 41.28 & 41.09 & 42.94 & 47.42 \\
32 & LISAC FSDM-USMBA & 47.36 & 36.58 & 36.27 & 39.32 & 44.00 \\
33 & YNU-HPCC & 29.95 & 25.31 & 25.31 & 25.21 & 28.52 \\
34 & IXA & 16.88 & 11.84 & 11.49 & 15.09 & 15.39 \\
\bottomrule

\end{tabular}%
} 
\caption{Detailed results for the English track.}
\label{tab:full_rank_en}
\end{table*}
