# Supplementary material for: SemEval-2023 Task 2: Fine-grained Multilingual Named Entity Recognition (MultiCoNER 2)
Source: arXiv:2305.06586 source file (2023-05-25)
Supplement: Supplementary file 3 [file f_r_es.tex]

\begin{table*}[!hbtp]
\resizebox{\textwidth}{!}{%
\begin{tabular}{c lllllll}

\toprule

\textbf{Rank} & 
\textbf{Team} & 
\textbf{Clean Subset F1} & 
\textbf{Noisy Subset F1} & 
\textbf{Entity Noise F1} &
\textbf{Context Noise F1} &  
\textbf{Macro F1}\\ 
\addlinespace[0.2cm]
\midrule

1 & DAMO-NLP & 91.74 & 85.81 & 85.29 & 91.06 & 89.78 \\
2 & CAIR-NLP & 85.03 & 80.66 & 80.44 & 82.92 & 83.63 \\
3 & USTC-NELSLIP & 77.25 & 68.52 & 68.00 & 73.73 & 74.44 \\
4 & IXA/Cogcomp & 77.65 & 66.09 & 65.48 & 72.30 & 73.81 \\
5 & Sakura & 75.42 & 67.39 & 66.93 & 72.01 & 72.85 \\
6 & NLPeople & 77.22 & 63.53 & 62.43 & 74.76 & 72.76 \\
7 & PAI & 79.35 & 55.25 & 53.16 & 75.10 & 71.67 \\
8 & BizNER & 72.60 & 69.11 & 69.08 & 69.53 & 71.48 \\
9 & garNER & 66.19 & 58.43 & 58.21 & 60.35 & 63.73 \\
10 & D2KLab & 66.69 & 55.75 & 55.26 & 60.47 & 63.17 \\
11 & silp\_nlp & 64.88 & 58.77 & 58.66 & 59.71 & 62.90 \\
12 & MEERQAT-IRIT & 63.04 & 56.42 & 56.16 & 58.78 & 60.93 \\
13 & LSJSP & 63.39 & 54.46 & 54.26 & 56.21 & 60.55 \\
14 & Sartipi-Sedighin & 62.27 & 50.25 & 49.70 & 55.57 & 58.41 \\
15 & LLM-RM & 57.42 & 49.32 & 49.19 & 50.47 & 54.81 \\
16 & FII\_Better & 58.96 & 44.77 & 43.57 & 56.07 & 54.51 \\
17 & SAB & 50.83 & 42.62 & 42.58 & 42.87 & 48.22 \\
18 & IXA & 17.65 & 12.16 & 11.83 & 14.59 & 16.01 \\
\bottomrule

\end{tabular}%
} 
\caption{Detailed results for the Spanish track.}
\label{tab:full_rank_es}
\end{table*}
