# Supplementary material for: SemEval-2023 Task 2: Fine-grained Multilingual Named Entity Recognition (MultiCoNER 2)
Source: arXiv:2305.06586 source file (2023-05-25)
Supplement: Supplementary file 4 [file f_r_fr.tex]

\begin{table*}[!hbtp]
\resizebox{\textwidth}{!}{%
\begin{tabular}{c lllllll}

\toprule

\textbf{Rank} & 
\textbf{Team} & 
\textbf{Clean Subset F1} & 
\textbf{Noisy Subset F1} & 
\textbf{Entity Noise F1} &
\textbf{Context Noise F1} &  
\textbf{Macro F1}\\ 
\addlinespace[0.2cm]
\midrule

1 & DAMO-NLP & 91.62 & 85.14 & 84.58 & 90.49 & 89.59 \\
2 & PAI & 89.50 & 78.71 & 77.64 & 88.96 & 86.17 \\
3 & CAIR-NLP & 84.67 & 79.54 & 79.22 & 82.55 & 83.08 \\
4 & BizNER & 79.09 & 75.63 & 75.29 & 78.92 & 78.01 \\
5 & IXA/Cogcomp & 78.60 & 65.81 & 64.93 & 74.14 & 74.52 \\
6 & USTC-NELSLIP & 76.81 & 68.49 & 67.93 & 73.55 & 74.25 \\
7 & Sakura & 75.58 & 66.86 & 66.38 & 71.26 & 72.86 \\
8 & NLPeople & 77.12 & 63.40 & 62.02 & 76.51 & 72.85 \\
9 & Ertim & 69.73 & 58.60 & 57.77 & 66.09 & 66.30 \\
10 & garNER & 68.09 & 60.22 & 59.77 & 64.27 & 65.68 \\
11 & D2KLab & 67.70 & 56.05 & 55.30 & 63.12 & 64.09 \\
12 & silp\_nlp & 64.40 & 58.04 & 57.81 & 60.02 & 62.39 \\
13 & MEERQAT-IRIT & 61.29 & 53.65 & 53.23 & 57.32 & 58.90 \\
14 & LSJSP & 58.74 & 52.60 & 52.34 & 54.93 & 56.83 \\
15 & SAB & 57.98 & 48.61 & 48.19 & 52.41 & 55.07 \\
16 & Sartipi-Sedighin & 56.99 & 50.40 & 50.22 & 52.05 & 54.94 \\
17 & IXA & 18.90 & 13.89 & 13.49 & 17.29 & 17.40 \\
\bottomrule

\end{tabular}%
} 
\caption{Detailed results for the French track.}
\label{tab:full_rank_fr}
\end{table*}
