# Supplementary material for: SemEval-2023 Task 2: Fine-grained Multilingual Named Entity Recognition (MultiCoNER 2)
Source: arXiv:2305.06586 source file (2023-05-25)
Supplement: Supplementary file 5 [file f_r_it.tex]

\begin{table*}[!hbtp]
\resizebox{\textwidth}{!}{%
\begin{tabular}{c lllllll}

\toprule

\textbf{Rank} & 
\textbf{Team} & 
\textbf{Clean Subset F1} & 
\textbf{Noisy Subset F1} & 
\textbf{Entity Noise F1} &
\textbf{Context Noise F1} &  
\textbf{Macro F1}\\ 
\addlinespace[0.2cm]
\midrule

1 & DAMO-NLP & 91.85 & 85.89 & 85.30 & 90.99 & 89.79 \\
2 & PAI & 88.94 & 76.53 & 75.14 & 89.56 & 84.88 \\
3 & CAIR-NLP & 85.08 & 81.00 & 80.58 & 84.63 & 83.78 \\
4 & BizNER & 77.24 & 74.81 & 74.34 & 79.33 & 76.48 \\
5 & USTC-NELSLIP & 78.06 & 70.65 & 70.05 & 75.91 & 75.70 \\
6 & IXA/Cogcomp & 78.16 & 67.66 & 66.77 & 75.95 & 74.67 \\
7 & Sakura & 76.67 & 69.03 & 68.53 & 73.18 & 74.19 \\
8 & NLPeople & 77.45 & 65.88 & 64.58 & 78.87 & 73.71 \\
9 & garNER & 70.16 & 63.99 & 63.53 & 67.81 & 68.20 \\
10 & D2KLab & 68.17 & 57.68 & 57.07 & 63.15 & 64.77 \\
11 & Sartipi-Sedighin & 67.61 & 57.95 & 57.16 & 65.31 & 64.50 \\
12 & silp\_nlp & 64.53 & 60.13 & 60.00 & 61.00 & 63.11 \\
13 & SAB & 60.36 & 51.60 & 51.15 & 55.56 & 57.57 \\
14 & FII\_Better & 60.32 & 47.85 & 46.76 & 58.36 & 56.36 \\
15 & IXA & 20.05 & 14.82 & 14.38 & 18.84 & 18.41 \\
\bottomrule

\end{tabular}%
} 
\caption{Detailed results for the Italian track.}
\label{tab:full_rank_it}
\end{table*}
