# Supplementary material for: SemEval-2023 Task 2: Fine-grained Multilingual Named Entity Recognition (MultiCoNER 2)
Source: arXiv:2305.06586 source file (2023-05-25)
Supplement: Supplementary file 6 [file f_r_pt.tex]

\begin{table*}[!hbtp]
\resizebox{\textwidth}{!}{%
\begin{tabular}{c lllllll}

\toprule

\textbf{Rank} & 
\textbf{Team} & 
\textbf{Clean Subset F1} & 
\textbf{Noisy Subset F1} & 
\textbf{Entity Noise F1} &
\textbf{Context Noise F1} &  
\textbf{Macro F1}\\ 
\addlinespace[0.2cm]
\midrule

1 & DAMO-NLP & 87.33 & 83.38 & 83.04 & 88.00 & 85.97 \\
2 & PAI & 84.56 & 76.12 & 75.50 & 82.87 & 81.61 \\
3 & CAIR-NLP & 81.73 & 77.10 & 76.94 & 78.61 & 80.16 \\
4 & BizNER & 74.36 & 70.35 & 70.12 & 72.81 & 72.97 \\
5 & IXA/Cogcomp & 76.00 & 65.54 & 64.91 & 72.32 & 72.28 \\
6 & USTC-NELSLIP & 74.04 & 65.91 & 65.49 & 70.37 & 71.26 \\
7 & Deep Learning Brasil & 72.07 & 68.91 & 68.75 & 70.11 & 70.97 \\
8 & NLPeople & 74.50 & 62.22 & 61.27 & 73.48 & 70.16 \\
9 & Sakura & 72.74 & 64.76 & 64.29 & 69.57 & 69.98 \\
10 & garNER & 66.81 & 60.04 & 59.82 & 61.52 & 64.51 \\
11 & Sartipi-Sedighin & 63.75 & 56.57 & 56.30 & 59.32 & 61.28 \\
12 & silp\_nlp & 63.07 & 57.23 & 56.99 & 59.93 & 61.05 \\
13 & D2KLab & 64.44 & 53.98 & 53.47 & 59.01 & 60.79 \\
14 & MEERQAT-IRIT & 61.82 & 56.17 & 56.01 & 58.00 & 59.87 \\
15 & LSJSP & 60.63 & 53.60 & 53.32 & 56.23 & 58.23 \\
16 & SAB & 57.55 & 47.56 & 47.21 & 51.08 & 54.12 \\
17 & IXA & 18.40 & 13.91 & 13.61 & 17.95 & 16.97 \\
\bottomrule

\end{tabular}%
} 
\caption{Detailed results for the Portuguese track.}
\label{tab:full_rank_pt}
\end{table*}
