# Supplementary material for: SemEval-2023 Task 2: Fine-grained Multilingual Named Entity Recognition (MultiCoNER 2)
Source: arXiv:2305.06586 source file (2023-05-25)
Supplement: Supplementary file 7 [file f_r_sv.tex]

\begin{table*}[!hbtp]
\resizebox{\textwidth}{!}{%
\begin{tabular}{c lllllll}

\toprule

\textbf{Rank} & 
\textbf{Team} & 
\textbf{Clean Subset F1} & 
\textbf{Noisy Subset F1} & 
\textbf{Entity Noise F1} &
\textbf{Context Noise F1} &  
\textbf{Macro F1}\\ 
\addlinespace[0.2cm]
\midrule

1 & DAMO-NLP & 91.08 & 86.76 & 86.34 & 91.41 & 89.57 \\
2 & CAIR-NLP & 84.54 & 79.75 & 79.49 & 80.75 & 82.88 \\
3 & IXA/Cogcomp & 80.75 & 68.69 & 67.99 & 74.81 & 76.54 \\
4 & BizNER & 77.23 & 73.87 & 73.54 & 77.78 & 76.12 \\
5 & USTC-NELSLIP & 78.51 & 69.64 & 69.22 & 72.87 & 75.47 \\
6 & NLPeople & 79.31 & 67.15 & 66.30 & 75.22 & 75.08 \\
7 & Sakura & 76.74 & 68.12 & 67.66 & 71.74 & 73.79 \\
8 & PAI & 81.53 & 55.22 & 53.04 & 77.04 & 72.38 \\
9 & garNER & 70.40 & 62.19 & 61.86 & 66.01 & 67.63 \\
10 & silp\_nlp & 67.15 & 60.87 & 60.53 & 63.74 & 65.00 \\
11 & LSJSP & 67.23 & 58.63 & 58.18 & 64.13 & 64.36 \\
12 & D2KLab & 66.78 & 55.80 & 55.29 & 61.14 & 62.98 \\
13 & Sartipi-Sedighin & 64.69 & 56.57 & 56.15 & 60.38 & 61.95 \\
14 & SAB & 61.58 & 51.14 & 50.90 & 52.90 & 58.03 \\
15 & FII\_Better & 56.66 & 43.11 & 42.20 & 50.67 & 52.12 \\
16 & IXA & 27.96 & 21.72 & 21.30 & 26.72 & 25.96 \\
\bottomrule

\end{tabular}%
} 
\caption{Detailed results for the Swedish track.}
\label{tab:full_rank_sv}
\end{table*}
