# Supplementary material for: SemEval-2023 Task 2: Fine-grained Multilingual Named Entity Recognition (MultiCoNER 2)
Source: arXiv:2305.06586 source file (2023-05-25)
Supplement: Supplementary file 8 [file f_r_zh.tex]

\begin{table*}[!hbtp]
\resizebox{\textwidth}{!}{%
\begin{tabular}{c lllllll}

\toprule

\textbf{Rank} & 
\textbf{Team} & 
\textbf{Clean Subset F1} & 
\textbf{Noisy Subset F1} & 
\textbf{Entity Noise F1} &
\textbf{Context Noise F1} &  
\textbf{Macro F1}\\ 
\addlinespace[0.2cm]
\midrule

1 & NetEase.AI & 88.47 & 69.05 & 67.80 & 86.43 & 84.05 \\
2 & DAMO-NLP & 82.91 & 54.32 & 52.26 & 81.45 & 75.98 \\
3 & SRCB & 87.19 & 39.39 & 35.37 & 88.37 & 75.86 \\
4 & PAI & 86.23 & 41.90 & 38.57 & 85.31 & 74.87 \\
5 & Taiji & 75.70 & 61.39 & 60.53 & 72.28 & 72.52 \\
6 & USTC-NELSLIP & 70.10 & 55.06 & 54.16 & 64.75 & 66.57 \\
7 & NLPeople & 71.43 & 48.95 & 47.91 & 61.57 & 65.96 \\
8 & IXA/Cogcomp & 70.35 & 48.37 & 47.36 & 59.88 & 64.86 \\
9 & Sakura & 68.79 & 51.20 & 50.43 & 59.73 & 64.61 \\
10 & garNER & 67.50 & 50.17 & 49.57 & 58.23 & 63.47 \\
11 & Ertim & 64.26 & 44.38 & 43.26 & 59.44 & 59.45 \\
12 & Sartipi-Sedighin & 62.60 & 46.46 & 46.10 & 49.10 & 58.70 \\
13 & CAIR-NLP & 62.89 & 44.74 & 43.84 & 56.16 & 58.43 \\
14 & Janko & 62.45 & 44.70 & 44.14 & 52.15 & 57.90 \\
15 & YNUNLP & 61.45 & 42.69 & 42.17 & 50.29 & 56.57 \\
16 & D2KLab & 58.75 & 43.34 & 42.67 & 48.12 & 54.92 \\
17 & silp\_nlp & 54.65 & 42.11 & 41.57 & 48.95 & 51.65 \\
18 & SAB & 47.71 & 33.37 & 32.46 & 42.82 & 44.12 \\
19 & NCUEE-NLP & 51.36 & 18.24 & 15.39 & 43.74 & 44.09 \\
20 & L3i++ & 38.02 & 27.13 & 26.63 & 32.99 & 35.34 \\
21 & YNU-HPCC & 34.24 & 24.07 & 23.52 & 32.50 & 31.66 \\
22 & IXA & 8.06 & 4.49 & 4.35 & 5.20 & 6.93 \\
\bottomrule

\end{tabular}%
} 
\caption{Detailed results for the Chinese track.}
\label{tab:full_rank_zh}
\end{table*}
